# Supplementary material for: Do causal predictors generalize better to new domains?
Source: arXiv:2402.09891 source file (2024-10-23)
Supplement: Supplementary file 1 [file mask.tex]

\begin{description}[font={\normalfont\itshape}]
    \item[Target:]
    \item[Shift:] 
    \item[List of causal features:]
    \begin{itemize}
        \item 
    \end{itemize}
   \item[List of arguably causal features:]
   \begin{itemize}
    \item 
    \end{itemize}
   \item[List of anticausal features:]
   \begin{itemize}
        \item
    \end{itemize}
   \item[List of other features:]
   \begin{itemize}
        \item
    \end{itemize}
\end{description}
    
\subcaptionbox{Out-of-domain accuracy}{
        \includegraphics[width = 0.3\textwidth]{figures/plots_empirical_results/plot_acsfoodstamps_ood_accuracy.pdf}
    }

\subcaptionbox{Balanced out-of-domain accuracy}{
    \includegraphics[width = 0.3\textwidth]{figures/plots_empirical_results/plot_acsfoodstamps_balanced_ood_accuracy.pdf}
    }
